# Supplementary material for: Triangle and Four Cycle Counting with Predictions in Graph Streams
Source: arXiv:2203.09572 source file (2022-03-17)
Supplement: Supplementary file 3 [file appendix.tex]

% \newpage
\section{Preliminaries}
In our analysis we use the following inequalities.

\begin{itemize}
    \item \textit{Chebyshev’s inequality.} Let $X$ be a random variable and $\epsilon > 0$. Then
    \[
    \textbf{Pr}[|X - \mathbb{E}[x]| \ge \epsilon] \le \frac{\textbf{Var}[X]}{\epsilon^2} \; .
    \]
    \item \textit{Chernoff’s bound.} Let $X_1, X_2,..., X_{\ell}$ be $\ell$ independent and identically distributed Bernoulli random variables with $\mathbb{E}[X_i] = \mu$ for each $i$. Then for any $\epsilon > 0$, we have 
    \[
    \textbf{Pr}[|\frac{1}{\ell} \sum_i X_i - \mu| \ge \epsilon \mu] \le 2e^ {-\epsilon^2 \mu \ell / 3} \; .
    \]
\end{itemize}

We will use exponential random variables in our analysis. 

\begin{definition}
An exponential random variable is parameterized by a parameter $\lambda$, denoted as $X \sim \mathrm{Exp}(\lambda)$. It has probability density function
\[
f(x)=\left\{\begin{array}{ll}
\lambda e^{-\lambda x}& \text{if } x \ge 0\\
0& \text{otherwise},
\end{array}\right.
\]
and cumulative density function
\[
F(x)=\left\{\begin{array}{ll}
1 - e^{-\lambda x}& \text{if } x \ge 0\\
0& \text{otherwise}.
\end{array}\right.
\]



\end{definition}
\section{Triangle Counting in the Adjacency List Model}
\label{appendix:B}
% \setlength\abovedisplayskip{2pt}
% \setlength\belowdisplayskip{2pt}

\subsection{Omitted proofs from Section~\ref{sec:adj_analysis}}

\textbf{Lemma~\ref{lem:adjlist_light}}
\textit{
Let $E$ be an edge set such that for each edge $xy \in E$, $R_{xy} \le \frac{T}{c}$, $T_L = \sum_{xy \in E} R_{xy} \le T$, and $S$ is a subset of $E$ such that every element in $E$ is included in $S$ independently with probability $\frac{1}{\rho}  = \alpha \epsilon^{-2} \frac{1}{c}$, for a sufficiently large constant $\alpha$. Then, with probability at least $9 / 10$, we have 
\[
\rho \sum_{xy \in S} R_{xy} = \sum_{xy \in E} R_{xy}  \pm \epsilon T \;.% +
\]
}

\begin{proof}
We let $Y = \rho \sum_{i \in S} R_{i} = \rho \sum_{i \in E} f_{i} R_{i}$, where $f_{i} = 1$ when $i \in S$ and $f_{i} = 0$ otherwise. It follows that $\mathbb{E}[Y] = T_L$. Then, 
\begin{align*}
\mathbf{Var}[Y]  =  &\mathbb{E}[Y^2] - {\mathbb{E}[Y]}^{2}  \\
& = \rho^2 \left( \mathbb{E}[ 
\sum \limits_{i \in E} {f_i R_i^2}  + \sum \limits_{i \neq j} f_i f_j R_i R_j ] \right) - T_{L}^2
\\
  & \le \rho^2 \left( \mathbb{E}[
\sum \limits_{i \in E} {f_i R_{i}^2}]  + \sum \limits_{i, j} \frac{1}{\rho^2} R_i R_j \right)  - T_{L}^2
  \\
  & = \rho \sum \limits_{i \in E} R_i^2
  \; .
\end{align*}

To bound this, we notice that $R_i \le \frac{T}{c}$ and $\sum_i R_i = T_L \le T$, so%{}%\setlength\abovedisplayskip{0.5pt} %\setlength\belowdisplayskip{2pt}
\[
\rho \sum \limits_{i \in E} R_i^2 \le \rho c (\frac{T}{c})^2 = \frac{\rho}{c} T^2 = \frac{1}{\alpha} \epsilon^2 T^2 \;.
\]
By Chebyshev's inequality, we have that 
\[
    \Pr [|Y - T_L| > \epsilon T] \le \frac{\frac{1}{\alpha}\epsilon^2 T^2}{\epsilon^2 T^2}\le \frac{1}{\alpha} \;. \qedhere
\]
\end{proof}

\textbf{Lemma~\ref{lem:adjlist_heavy}}
\textit{
Let $xy$ be an edge in $E$. We sample the edges with rate $\frac{1}{\rho} = \beta \epsilon^{-2} \log n/ c$ in the stream for a sufficiently large constant $\beta$. Consider 
\[
\# = |xz \textnormal{ has been sampled}: \{x, y, z\} \in \Delta \textnormal{ and } x <_s z <_s y| \; .
\]
Then we have the following: if $R_{xy} \ge \frac{c}{2}$, then with probability at least $1 - \frac{1}{n^5}$, we have $\rho \# = (1 \pm \epsilon) R_{xy}$. If $R_{xy} < \frac{c}{2}$, then with probability at least $1 - \frac{1}{n^5}$, we have $ \# <  c / \rho$.
}
\begin{proof}
We first consider the case when $R_{xy} \ge \frac{c}{2}$.

For each edge $i \in |xz : \{x, y, z\} \in \Delta \textnormal{ and } x <_s z <_s y|$, let $X_i$ = 1 if $i$ has been sampled, or $X_i = 0$ otherwise. We can see the $X_i$ are i.i.d. Bernoulli random variables and $\mathbb{E}[X_i] = 1/\rho$. By a Chernoff bound we have
\[
\mathbf{Pr}[|\sum_i X_i - \frac{1}{\rho} R_{xy}| \ge \epsilon \frac{1}{\rho} R_{xy}] \le 2e^{-\epsilon^2 \frac{1}{\rho} R_{xy}/3} \le \frac{1}{n^5} \; .
\]
Therefore, we have
\begin{align*}
\mathbf{Pr}[|\rho \# - R_{xy}| \ge \epsilon R_{xy}] =& \mathbf{Pr}[ |\rho \sum_i X_i - R_{xy}| \ge \epsilon R_{xy}] \\
&\le \frac{1}{n^5} \; .
\end{align*}
Alternatively, when $R_{xy} < \frac{c}{2}$, we have 
\[
 \mathbf{Pr}[|\rho \# - R_{xy}| \ge \frac{1}{2}c] \le \frac{1}{n^5} \; ,
\]
which means $\rho \# < c$ with probability at least $1 - \frac{1}{n^5}$.
\end{proof}
\textbf{Theorem~\ref{theorem_adjacency}}
\textit{
There exists a one-pass algorithm with $\tilde{O}( \min(\epsilon^{-2}m^{2/3}/T^{1/3}, \epsilon^{-1} m^{1/2}))$ memory in the adjacency list model using a learning-based oracle that returns a $(1 \pm \epsilon)$-approximation to $T$ with probability at least $7 / 10$. 
}

\begin{proof}
We first consider the case when $T \ge (m / \epsilon)^{1/2}$.

For each edge $xy \in H$, from Lemma~\ref{lem:adjlist_heavy} we have that with probability at least $1 - \frac{1}{n^5}$, $\# / p_3 = (1 \pm \epsilon) R_{xy}$ in Algorithm~\ref{alg:1}. If $xy \notin H$, then with probability $1 - \frac{1}{n^5}$, $xy$ will not contribute to $A_h$. Taking a union bound, we have that with probability at least $1 - 1/n^3$, 
\[
A_h / p_3 = (1 \pm \epsilon) \sum_{xy \in H} R_{xy} = (1 \pm \epsilon) T_H \; .
\]
For the medium edges and light edges, we notice that a medium edge $xy$ satisfies $R_{xy} \le \rho = T / (T / \rho)$ and a light edge $xy$ satisfies $R_{xy} \le T / \rho$. From Lemma~\ref{lem:adjlist_light} we have that with probability $4/5$,
\[
A_m / p_2 = T_M \pm \epsilon T,  A_l / p_1 = T_L \pm \epsilon T\; .
\]
Putting everything together, we have that with probability $7/10$,
\[
|A_h / p_3 + A_m / p_2 + A_l / p_1 - T| \le 3 \epsilon T.
\]
%which is our need. 
Now we analyze the space complexity. We note that there are at most $\rho$ medium edges. Hence, the expected total space we use is
$O(m p_3 + \rho p_2 + m p_1) = O(\epsilon^{-2} m^{2/3} / T^{1/3}\log n)$\footnote{Using Markov's inequality, we have that with probability at least $9 / 10$, the total space we use is less than $10$ times the expected total space.}. 

When $T < (m / \epsilon)^{1/2}$, as described in Section~\ref{sec:adjacency_list_intuition}, we only have two classes of edges: heavy and light. We will save all the heavy edges and use sub-sampling to estimate $T_L$. The analysis is almost the same.
\end{proof}

\textbf{Theorem~\ref{thm:adj_noisy}}
\textit{
With a noisy heavy edge oracle, which errs with probability $\delta$, we can obtain a $(1 \pm \epsilon)$-approximation to the number of triangles in the adjacency list model with space complexity $\tilde{O}(\epsilon^{-2} \min(m^{2/3} / T^{1/3}, m^{1/2}))$ when $\delta = O(T^{1/3} / m^{2/3})$, or with space complexity $\tilde{O}(\epsilon^{-2} \min(m\delta^{1/2} / T^{1/2}, m \delta))$ otherwise. Both guarantees hold with success probability at least $7/10$.
}

\begin{proof}
%Note that we do not use the oracle to distinguish between heavy and medium edge. Hence
Let $L_O$ be the set of edges that the oracle predicts are the light edges. By assumption, we get that for every edge $xy$ in $L_O$, with probability at least $1-\delta$, $R_{xy} \le \frac{T}{\rho}$, and with probability $\delta$, $R_{xy} \le \rho$ (because we can detect the heavy edges without the oracle).

Similar to the proof in Section~\ref{lem:adjlist_light}, we have 
\begin{align*}
\mathbf{Var}[A_l / p_3] &= \gamma \epsilon^{2} \rho  \mathbb{E} [\sum_{i \in L_O} R_i^2] \\
&\le \gamma \epsilon^{2}\rho ((1 - \delta) \rho \frac{T^2}{\rho^2} + \delta \rho^2 \frac{T}{\rho}) \\
&= \gamma \epsilon^{2} ((1 - \delta)T^2 + \delta \rho^2 T).
\end{align*}
Hence, we have that when $\delta \rho^2 < T$, $\mathbf{Var}[A_l / p_3] \le \gamma \epsilon^{2} T^2$, where the condition is equivalent to $\delta = O(T^{1/3} / m^{2/3})$ (recall $\rho = (mT)^{1/3}$).

When $\delta = O(T^{1/3} / m^{2/3})$, in expectation there will be at most $m \delta = O(\rho)$ light edges that will be classified as medium edges. Hence, when $\delta = O(T^{1/3} / m^{2/3})$, the guarantee of Theorem~\ref{theorem_adjacency} still holds.

When $\delta = \Omega(T^{1/3} / m^{2/3})$, from the above analysis we can instead set $\rho = (T / \delta)^{1/2}$ and define the edge $xy$ to be heavy if $R_{xy} \ge \rho$, light if $R_{xy} \le \frac{T}{\rho}$, and medium if $\frac{T}{\rho} < R_{xy} < \rho$. In this case, the guarantee of Theorem~\ref{theorem_adjacency} will still hold and the space will become $\tilde{O}(m\delta^{1/2} / T^{1/2})$.

On the other hand, similar to the case when $T < (m / \epsilon)^{1/2}$, we can also set an edge to be heavy if $R_{xy} \ge m \delta$, and light otherwise. We then save all of the heavy edges and use sub-sampling with rate $O(\epsilon^{-2} / \delta)$ to estimate $T_L$. The space used will become $O(\epsilon^{-2} m \delta)$, which means we can get an $\tilde{O}(\epsilon^{-2} \min(m\delta^{1/2} / T^{1/2}, m \delta))$ space algorithm when $\delta = \Omega(T^{1/3} / m^{2/3})$.
\end{proof}

\subsection{Algorithm with a Value Prediction Oracle}

In this section, we consider the following oracle model.

\textbf{Definition~\ref{def:value_oracle}}
\textit{
A heavy edge oracle with parameter $(\alpha,\beta)$ can, for a given edge $xy$, indicate if (i) $R_{xy} \le T / \beta$, or (ii) $R_{xy} > T / \beta$, and output a value  $\hat{R}_{xy}$ for which $\alpha R_{xy} \ge \hat{R}_{xy} \ge R_{xy}$.
%$\alpha$-approximation of $R_{xy}$ .
}

Our algorithm is based on the following stability property of exponential random variables (see e.g.~\cite{Andoni17})

\begin{lemma}
\label{lem:exp_stable}
Let $x_1, x_2, ..., x_n > 0$ be real numbers, and let $u_1, u_2, ...u_n$ be i.i.d. standard exponential random variables with parameter $\lambda = 1$. Then we have that the random variable $\max(\frac{x_1}{u_1}, ..., \frac{x_n}{u_n}) \sim \frac{x}{u}$, where $x = \sum_i x_i$ and $u \sim \mathrm{Exp}(1)$.
\end{lemma}

\begin{lemma}
\label{lem:exp_median}
Let $r = O(\ln(1 / \delta) / \epsilon^{2})$ and $\epsilon \le 1/3$. If we take $r$ independent samples $X_1, X_2, ... , X_r$ from $\mathrm{Exp}(1)$ and let $X = \mathrm{median}(X_1, X_2, ..., X_r)$, then with probability $1 - \delta$, $X \in [\ln{2}(1-\epsilon), \ln{2}(1 + 5\epsilon)]$.
\end{lemma}
\begin{proof}
We first prove the following statement: with probability $1-\delta$, $F(X) \in [1/2-\epsilon, 1/2 + \epsilon]$, where $F$ is the cumulative density function of a standard exponential random variable.

Consider the case when $F(X) \le 1/2 - \epsilon$. We use the indicator variable $Z_i$ where $Z_i = 1$ if $F(X_i) \le 1/2 - \epsilon$ or $Z_i = 0$ otherwise. Notice that when $F(X) \le 1/2 - \epsilon$, at least half of the $Z_i$ are $1$, so $Z = \sum_i Z_i \ge r / 2$. On the other hand, we have $\mathbb{E}[Z] = r / 2 - r \epsilon$, by a Chernoff bound. We thus have 
\[
\mathbf{Pr}[|Z - \mathbb{E}[Z]| \ge \epsilon r] \le 2e^{-\epsilon^{2}r/3} \le \delta / 2\; .
\]
Therefore, we have with probability at most $\delta/2$, $F(X) \le 1/2 - \epsilon$. Similarly, we have that with probability at most $\delta / 2$, $F(X) \ge 1/2 + \epsilon$. Taking a union bound, we have that with probability at least $1-\delta$, $F(X) \in [1/2-\epsilon, 1/2 + \epsilon]$.

Now, condition on $F(X) \in [1/2-\epsilon, 1/2 + \epsilon]$. Note that $F^{-1}(x) = -\ln(1 - x)$, so if we consider the two endpoints of $F(X)$, we have 
\[
F^{-1} (1/2 -\epsilon) = -\ln(1/2 + \epsilon) \ge (1-\epsilon)\ln{2},
\]
and
\[
F^{-1} (1/2 +\epsilon) = -\ln(1/2 - \epsilon) \le (1+5\epsilon)\ln{2}.
\]
which indicates that $X \in [\ln{2}(1-\epsilon), \ln{2}(1 + 5\epsilon)]$.
\end{proof}

The algorithm is shown in Algorithm~\ref{alg:4}. For the light edges, from the assumption of the oracle we know that $R_{xy} \le T / \beta$, we can sub-sample with sampling rate $O(\epsilon^{-2} \beta)$ to estimate $T_L$. For the heavy edges, we can obtain an $\alpha$-approximation to $R_{xy}$ from the oracle at this time. As shown in our algorithm, we run $O(\epsilon^{-2})$ copies of the subroutine and we will show that each subroutine will output the maximum value of $R_{xy} / u_{xy}^i$ with high probability, where the $u_{e}^i$ are exponential random variables. From Lemma~\ref{lem:exp_stable} and Lemma~\ref{lem:exp_median} we can obtain $O(\epsilon^{-2})$ independent samples from $T_H / u$, where $u \sim \mathrm{Exp}(1)$, and after taking a median among all samples we can obtain a $(1 \pm \epsilon)$-approximation to $T_H$.

\begin{algorithm}[!h]
   \caption{Counting Triangles in the Adjacency List Model with a Value Prediction Oracle}
   \label{alg:4}
\begin{algorithmic}[1]
   \STATE {\bfseries Input:} Adjacency list edge stream and an oracle that outputs \textsc{true} if $R_{xy} \le T / \beta$ and \textsc{false} with an $\alpha$-approximation to $R_{xy}$.
   \STATE {\bfseries Output:} An estimate of the number $T$ of triangles.
   \STATE Initialize $A_l \leftarrow 0, S_L \leftarrow \emptyset$ and set $p_l \leftarrow \gamma \epsilon^{-2}/\beta$. $X \leftarrow \emptyset$ and $k \leftarrow l \alpha$ for a sufficiently large constant $l$\; .
   %\STATE On :
   \FOR{$i = 0$ {\bf to} ${O(\epsilon^{-2})}$}
        \STATE $S^{i} \leftarrow \emptyset, Q^{i} \leftarrow \emptyset$, and $A^i \leftarrow 0 $ \; .
        % \STATE $v_i \leftarrow 0$ \textnormal{as the maximum value in $Q^i$} \; .
        % \STATE $w_i \leftarrow 0$ \textnormal{as the minimum value in $Q_i$} \;%\textnormal{as the evict threshold in $Q^i$} 
        \STATE \textnormal{Generate} $u_{xy}^i \sim \textrm{Exp}(1)$ for all $x$ and $y$ \; . 
   \ENDFOR
    \WHILE{seeing edges adjacent to $y$ in the stream} \STATE For all $ab \in S_L$: if $a, b \in N(y)$ then $C_{ab} \leftarrow C_{ab} + 1$\; 
    % \FOR{$i = 0$ {\bf to} ${O(\epsilon^{-2})}$}
    \STATE For all $ab \in S^i$: if $a, b \in N(y)$ then $C_{ab}^i \leftarrow C_{ab}^i + 1$\; 
    %  \ENDFOR
    \FOR{each incident edge $yx$}
    
    \IF{the oracle outputs \textsc{True}}
    \IF{$xy \in S_L$} 
        \STATE $A_l \leftarrow A_l + C_{xy}$ \;.
    \ELSE 
    \STATE With probability $p_l$, $S_L \leftarrow \{yx\} \cup S_L$ \;.
    \ENDIF
    \ELSE 
        \FOR{$i = 0$ {\bf to} ${O(\epsilon^{-2})}$} 
            \IF{$xy \in S^i$} 
            \STATE $A^i \leftarrow \max(A^i,  C_{xy}^i / u_{xy}^i)$ \;.
            \ELSE
            \STATE Let $\hat{R}_{yx}$ be the predicted value of $R_{yx}$.
            \STATE $Q^i \leftarrow Q^i \cup \{\hat{R}_{yx}/u_{yx}^i\}, S^i \leftarrow S^i \cup \{xy\}$
            \IF{$|Q| > k$}
            \STATE Let $ab$ be the edge for which $\hat{R}_{ab} / u_{ab}^i$ is the smallest item in $Q^i$
            \STATE $Q^i \leftarrow Q^i / \{\hat{R}_{ab}/u_{ab}^i\}, S^i \leftarrow S^i / \{ab\}$
            \ENDIF
            \ENDIF
    \ENDFOR
    
    \ENDIF
    \ENDFOR
    \ENDWHILE
    \FOR{$i = 0$ {\bf to} ${O(\epsilon^{-2})}$}
        \STATE $u^i \leftarrow \max(Q^i)$ and $v^i \leftarrow \min(Q^i)$  \; .
        \IF{$u^i > \alpha v^i$}
        \STATE $X \leftarrow X \cup \{A^i\}$
        \ENDIF
   \ENDFOR
    \STATE {\bfseries return:} $A_l / p_l + \mathrm{median}(X) / \ln{2}$ \; .
\end{algorithmic}
\end{algorithm}

\textbf{Theorem~\ref{thm:value_oracle}}
\textit{
Given an oracle with parameter $(\alpha, \beta)$, there exists a one-pass algorithm with space complexity $O(\epsilon^{-2} (m / \beta + \alpha + \log n(\log\log n)^2))$ in the adjacency list model that returns a $(1 \pm \epsilon)$-approximation to $T$ with probability at least $7 / 10$. 
}

\begin{proof}
For the light edges, from Lemma~\ref{lem:adjlist_light} we get that with probability at least $9/10$, 
\[
A_l / p_l = T_L \pm \epsilon T \;.
\]
Now we focus on estimating $T_H$. It is easy to see that for the $i$-th subroutine, $Q^i$ and $S^i$ sample the edge $xy$ for which $\hat{R}_{xy} / u_{xy}^i$ is among the current top $k$ values we have seen. At the end of the stream, $Q^i$ and $S^i$ sample edge $xy$ for which $\hat{R}_{xy} / u_{xy}^i$ is among the top $k$ largest values among all edges. If the edge $ab$, for which the true value $R_{ab} / u_{ab}^i$ is the maximum value among $E$, is included in $S^i$, then the output of the $i$-th subroutine will be a sample from $T_H / u$, where $u \sim \mathrm{Exp}(1)$. Recall that $\hat{R}_{xy}$ is an $\alpha$-approximation to $R_{xy}$, and hence we have that 
\[
\max_{xy \in E} \hat{R}_{xy} / u_{xy}^i \le \alpha \hat{R}_{ab} / u_{ab}^i \;,
\]
which means if $u_i \ge \alpha v_i$ ($u_i$ and $v_i$ are the maximum and minimum values in $Q^i$ after the stream), then $ab$ should be included in $S^i$.

From Claim~2.1 in~\cite{Andoni17}, for each subroutine $i$, in expectation there will be at most $O(\alpha)$ edges $wz$ satisfying 
\[
\max_{xy \in E} \hat{R}_{xy} / u_{xy}^i \le \alpha \hat{R}_{wz} / u_{wz}^i \;,
\]
Hence, using Markov's inequality, with probability at least $9 / 10$, $u_i > \alpha v_i$ holds for the $i$-th subroutine (this is because, at this time there are at most $O(\alpha)$ edges within an $\alpha$ factor of $\max_{xy \in E} \hat{R}_{xy} / u_{xy}^i$, and $v_i$ is the $k = l \alpha$ largest edge). Therefore, in expectation there will be at least a $9/10$-fraction of our total  $O(\epsilon^{-2})$ number of subroutines which can output a sample drawn from $T_H / u$. From Lemma~\ref{lem:exp_median}, we get that after taking a median, we obtain a $(1 \pm O(\epsilon))$-approximation to $T_H$.

Next we analyze the space complexity. For the light edges, we sample each edge with probability $O(\epsilon^{-2}/\beta)$, and hence the expected space we use is $O(\epsilon^{-2} m / \beta)$. For the heavy edges, we run $O(1/\epsilon^{2})$ subroutines and the number of edges each subroutine stores is $O(\alpha)$. From Theorem~5 in \cite{JW18}, generating the exponential random variables can be derandomized in $O(\epsilon^{-2} (\log n (\log\log n)^2))$ space. Therefore, we get that the total expected space we use is $O(\epsilon^{-2}(m / \beta + \alpha + \log n (\log\log n)^2))$.
\end{proof}

\begin{remark}
An alternative way to solve this problem is to divide the triangles into the intervals $[0, T/\beta], [2T/ \beta, 4T/ \beta],..., [2^i T/\beta, 2^{i+1} T / \beta], ...$ and put the edges into the intervals according to the predicted value the oracle gives. For the edges in interval $[2^i T / \beta, 2^{i + 1} T / \beta]$, we can sub-sample with rate $O(\epsilon^{-2} \alpha 2^{i + 1} /\beta )$. The total space we use will be $\tilde{O}(\epsilon^{-2} (m / \beta + \alpha \log n))$.
\end{remark}
\section{Triangle Counting in the Arbitrary Order Model}
\label{appendix:C}
\subsection{Omitted proof in Section~\ref{sec:arbitrary_triangle_analysis}}
From~\cite{MVV16}, we have the following analysis.
\begin{lemma}[\cite{MVV16}]
\label{lem:arbitrary_light}
For the edge sampling algorithm shown in Section~\ref{sec:arbitrary_triangle_intuition}, we have
\[
\mathbf{Pr}[|\frac{C}{p^2} - T| \ge \epsilon T] \le \frac{T + Tp\Delta_E}{\epsilon^2 T^2 p^2} \; .
\]
\end{lemma}

\textbf{Theorem~\ref{theorem_arbitrary}}
\textit{
There exists a one-pass algorithm with space complexity $\tilde{O}(\epsilon^{-2}\max(m/\sqrt{T}, \sqrt{m}))$ in the arbitrary order model using a learning-based oracle that returns a $(1 \pm \epsilon)$-approximation to $T$ with probability at least $7 / 10$. 
}

\begin{proof}
We first consider the case when $T \le m$. For the light edges, recall the threshold is $N_{uv} \le 2\sqrt{T}$ and we sample the edges with probability $\alpha \epsilon^{-2} / \sqrt{T}$. Hence from Lemma~\ref{lem:arbitrary_light}, we obtain a $(1 \pm \epsilon)$-approximation to $T_L$ with probability at least $9/10$, where $T_L$ denotes the number of triangles having three light edges. 

Now we consider estimating $T_H$, where $T_H$ is the number of triangles that have at least one heavy edge. Given a heavy edge $uv$, we define $N_{uv}^i$ to be the number of triangles that share edge $uv$ and have exactly $i$ heavy edges ($i = 1, 2, 3$). It is easy to see that
\[
\sum_{uv \in H} (N_{uv}^1 + 1/2 N_{uv}^2 + 1/3 N_{uv}^3) = T_H \;.
\]
Note that we store all the heavy edges, and hence we can compute the exact value of $N_{uv}^3$. There are at most $3\sqrt{T}/2$ heavy edges, so $N_{uv}^2 + N_{uv}^3 \le 3\sqrt{T}/2$, which makes $N_{uv}^1 \ge \sqrt{T} / 2$. As in the proof of Lemma~\ref{lem:adjlist_light}, using a vertex sampling method we can obtain a $(1 \pm \epsilon)$-approximation to $N_{uv}$ and to $N_{uv}^1$ (we denote these by $\hat{N}_{uv}$ and $\hat{N}_{uv}^1$). Let $\hat{N}_{uv}^2 = \hat{N}_{uv} - \hat{N}_{uv}^1 - N_{uv}^3$, one can show that 
\[
\hat{N}_{uv}^1 + 1/2 \hat{N}_{uv}^2 + 1/3 \hat{N}_{uv}^3 = (1 \pm 2\epsilon) (N_{uv}^1 + 1/2 N_{uv}^2 + 1/3 N_{uv}^3) \;.
\]
Taking a union bound, we obtain a $(1 \pm 2\epsilon)$-approximation to $T_H$ with probability at least $9 / 10$.

Now we analyze the space complexity. For the light edges we sample, the expected space is $O(pm) = O(\epsilon^{-2} m / \sqrt{T})$. For the vertices with the incident edges that we sample, the expected space is $O(p \sum_v \mathrm{deg}(v)) = O(p \cdot 2m) = \tilde{O}(\epsilon^{-2} m / \sqrt{T})$. Additionally, there are at most $O(\sqrt{T})$ heavy edges, and so we get that the expected total space is $\tilde{O}(\epsilon^{-2} m / \sqrt{T})$.

When $T > m$, the threshold for heavy edges becomes $N_{uv} \ge 2 T / \sqrt{m}$ and the sampling rate becomes $\tilde{O}(\epsilon^{-2} / \sqrt{m})$. The analysis then proceeds as before.
\end{proof}

\textbf{Theorem~\ref{thm:arbitrary_noise}}
\textit{
With a noisy heavy edge oracle with error probability $\delta$, we can estimate the number of triangles within a factor of $(1 \pm \epsilon)$ in the arbitrary order model with space complexity $\tilde{O}(\epsilon^{-2}\max(m/\sqrt{T}, \sqrt{m}))$ when $\delta = O(\frac{T}{\Delta_E}\max(\frac{1}{\sqrt{T}}, \frac{1}{\sqrt{m}}))$, or with space complexity $\tilde{O}(\epsilon^{-2}(\max(m/\sqrt{T}, \sqrt{m}) + \delta m \Delta_E / T))$ otherwise. Both guarantees hold with success probability at least $7/10$.
}
\begin{proof}
We note that for a light edge $uv$, which can be classified as a heavy edge, we can detect this after the stream using the vertices with incident edges that we sampled. Hence, we only need to consider the case when a heavy edge is classified as a light edge (during the stream we can sample each edge with probability $p$ and save all the triangles we found. Then, after the stream, we can check whether the triangles contain heavy edges or not).

For the estimation of $T_L$, similar to the proof in Theorem~\ref{thm:arbitrary_noise} and Lemma~\ref{lem:arbitrary_light}, we have
\[
\textbf{Var}[A]  \le p^2 T + (1-\delta) p^3 \rho T  + \delta p^3 \Delta_E T\; ,
\]
where $\rho = T / \min(\sqrt{T}, \sqrt{m})$. Hence when $\delta \Delta_E \le \rho$, the third term is bounded by the second term, which ensures that the guarantee of Theorem~\ref{theorem_arbitrary} still holds. 

When $\delta \Delta_E > \rho$, to bound the third term, the edge sampling rate $p$ should be $\Omega(\epsilon^{-2}\Delta_E / T)$, which will make the space we use become $\tilde{O}(\epsilon^{-2}(\max(m/\sqrt{T}, \sqrt{m}) + \delta m \Delta_E / T))$.
\end{proof}
\subsection{Lower Bound}

In this section, we give our lower bound for the space complexity in the arbitrary order model with the help of a heavy edge oracle. As described in Section~\ref{sec:lower_bound}, we assume the threshold $c = o(m)$ and $T / c > 1$, as otherwise the threshold will be too small or too close to the average to provide an accurate prediction. 

When $T \le m$, we consider the hubs graph mentioned in~\cite{KP17}.

\begin{definition}[Hubs Graph, \cite{KP17}]
The hubs graph $H_{r,d}$ consists of a single vertex $v$ with $2rd$ incident edges, and $d$ edges connecting disjoint pairs of $v$’s neighbors to form triangles.
\end{definition}

It is easy to see that in $H_{r, d}$, each edge has at most one triangle. Hence, there will not be any heavy edges of this kind in the graph. In~\cite{KP17}, the authors show an $\Omega(r\sqrt{d})$ lower bound for the hubs graph.

\begin{lemma}[\cite{KP17}]
Given $r$ and $d$, there exist two distributions $\mathcal{G}_1, \mathcal{G}_2$ on subgraphs $G_1$ and $G_2$ of $H_{r, d}$, such that any algorithm which distinguishes them with probability at least $2/3$ requires $\Omega(r\sqrt{d})$ space, where $G_i$ has $\Theta(rd)$ edges and $T(G_1) = d, T(G_2) = 0$.
\end{lemma}

Now, given $T$ and $m$, where $T \le m$, we let $r = \Theta(m/T)$ and $d = T$. We can see $H_{r, d}$ has $\Theta(m)$ edges and $T$ triangles, and we need $\Omega(r\sqrt{d}) = \Omega(m / \sqrt{T})$ space. 

When $T > m$, we consider the following $\Omega(m^{3/2} /  T)$ lower bound in~\cite{BC17}. % hard instances

Let $H$ be a complete bipartite graph with $b$ vertices on each side (we denote the two sides of vertices by $A$ and $B$). We add an additional $N$ vertex blocks $V_1, V_2, ... V_N$  with each $|V_i| = d$. Alice has an $N$-dimensional binary vector $x$. Bob has an $N$-dimensional binary vector $y$. Both $x$ and $y$ have exactly $N/3$ coordinates that are equal to $1$. Then, we define the edge sets 
\[
E_{\mathrm{Alice}} = \bigcup_{i:x_i = 1} \{\{u, v\}, u \in A, v \in V_i\}
\]
and
\[
E_{\mathrm{Bob}} = \bigcup_{i:y_i = 1} \{\{u, v\}, u \in B, v \in V_i\} \; .
\]
Let the final resulting graph be denoted by $G = (V, E)$ where $V = V_H \cup V_1 \cup ... \cup V_N$ and $E = E_H \cup E_{\mathrm{Alice}} \cup E_{\mathrm{Bob}}$.

In~\cite{BC17}, the authors show by a reduction to the $\textsc{DISJ}_N^{N/3}$ problem in communication complexity, that we need $\Omega(N)$ space to distinguish the case when $G$ has $0$ triangles from the case when $G$ has at least $b^2d$ triangles.

Given $m$ and $T $, $ T = \Theta(m^{1 + \delta})$ where $1 \le \delta < 1/2$, as shown in~\cite{BC17}, we can set $b = N^{s}$ and $d = N^{s - 1}$ where $s = 1/(1 - 2\delta)$. This will make $m = \Theta(N^{2s})$ and $T = \Theta(N^{3s - 1})$, which will make the $\Omega(m^{3/2} / T)$ lower bound hold. Note that at this time each edge will have an $O(\frac{1}{m})$-fraction of triangles or  an $O(\frac{1}{m^{1-\frac{1}{2s}}})$-fraction of triangles. Assume the threshold of the oracle $c = O(m^q)$. When $\delta \ge \max(0, q - \frac{1}{2})$, there will be no heavy edges in the graph.

Putting everything together, we have the following theorem.

\textbf{Theorem~\ref{thm:lower_bound_arbitrary}}
\textit{
Suppose that the threshold of the oracle $c = O(m^q)$, where $0 \le q < 1$. Then for any $T$ and $m$, $T \le m$, there exists $m^\prime = \Theta(m)$ and $T^\prime = \Theta(T)$ such that any one-pass arbitrary order streaming algorithm that distinguishes between $m^\prime$ edge graphs with $0$ triangles versus $T^\prime$ triangles, with probability at least $2/3$, requires $\Omega(m / \sqrt{T})$ space. For any $T$ and $m$, $T = \Omega(m^{1 + \delta})$ where $\max(0, q - \frac{1}{2}) \le \delta < \frac{1}{2}$, there exists $m^\prime = \Theta(m)$ and $T^\prime = \Theta(T)$ for which any one-pass arbitrary order streaming algorithm that distinguishes between $m^\prime$ edge graphs with $0$ triangles versus $T^\prime$ triangles, with probability at least $2/3$, requires $\Omega(m^{3/2} / T)$ space.
}
\section{Four-Cycle Counting in the Arbitrary Order Model}
\label{appendix:D}


\textbf{Theorem~\ref{theorem_four_cycle}}
\textit{
There exists a one-pass algorithm with space complexity $\tilde{O}(T^{1 / 3} + \epsilon^{-2}m / T^{1/3})$ in the arbitrary order model using a learning-based oracle that returns a $(1 \pm \epsilon)$-approximation to $T$ with probability at least $7 / 10$. 
}

\begin{proof}
From the Lemma 3 in ~\cite{SV20}, we know that with probability at least $9/10$, we can get an estimate $A_w$ such that
\[
A_w = T_w \pm \epsilon T.
\]
Where $T_w$ is the number of the 4-cycles that have at least one heavy wedge. We note that if a 4-cycle has two heavy wedges, it will be counted twice. However, \cite{SV20} shows that this double counting is at most $O(T^{2/3}) = O(\epsilon)T$. 

For the edge sampling algorithm mentioned in~\ref{sec:four_cycle_intuition}, from the analysis in~\cite{SV20}, we have 
\[
\textbf{Var}[\frac{A_l}{p^3}] \le O(T / p^3 + T\Delta_E / p + T\Delta_W / p^2)\; .  
\]
Notice that in our algorithm, the threshold of the heavy edges and heavy wedges are $N_{uv} \ge T^{2/3}$ and $N_w \ge T^{1/3}$, respectively, which means $\textbf{Var}[\frac{A_l}{p^3}] = O(\epsilon^2 T^2)$. Hence, we can get an estimate $A_l$ such that with probability at least $9/10$, 
\[
A_l = T_l \pm \epsilon T\;,
\]
where $T_l$ is the number of 4-cycles that have no heavy edges. 
Similarly, we have with probability at least $9/10$, 
\[
A_h = T_h \pm \epsilon T\;,
\]
where $T_h$ is the number of 4-cycles that have at most one heavy edge.

One issue is that the algorithm has not yet estimated the number of 4-cycles having more than one heavy edge, but without heavy wedges. However, from Lemma 5.1 in~\cite{McGregor2020} we get that the number of this kind of 4-cycles is at most $O(T^{5/6}) = O(\epsilon)T$. Hence putting everything together, we have
\[
|A_l/p^3 + A_h/p^3 + A_w - T| \le O(\epsilon) T \;,
\]
which is what we need.

Now we analyze the space complexity. The expected number of light edges we sample is $O(mp) = \tilde{O}(\epsilon^{-2} m / T^{1/3})$ and the expected number of nodes in $S$ and edges in $E_S$ is $O(2mp) = \tilde{O}(\epsilon^{-2} m / T^{1/3})$. The expected number of 4-cycles we store in $D$ is $O(T p^3) = \tilde{O}(\epsilon^{-6})$. We store all the heavy edges, and the number of heavy edges is at most $O(T^{1/3})$. Therefore, the expected total space is $\tilde{O}(T^{1 / 3} + \epsilon^{-2}m / T^{1/3})$.
\end{proof}


\section{Accuracy of the Oracle}
\label{appendix:E}

In this section, we evaluate the accuracy of the predictions the oracle gives in our experiments. We assess it from two perspectives: (i) given the top $k$ edges that the oracle predicts, how many of them are indeed among the top $k$ edges? (ii) for the top $k$ edges the oracle predicts (we use $S_k$ to denote the set of these edges), how close is the predicted value to the true value?

The results are shown in Table~\ref{table:1} for $k = 50, 100, 200, 500$ and $1000$. Here we use $\rho_k$ to denote the average multiplicative error for $R_{uv}$ over $S_k$ in the adjacency list model or for $N_{uv}$ in the arbitrary order model. 
We can see in the adjacency list model, the accuracy of the top $k$ edges is above $80\%$ for both networks when $k \le 1000$ and when $k$ is small we can get a good approximation to $R_{uv}$. 
In the arbitrary order model, we can see that as the value $k$ becomes larger, both the accuracy and $\rho_k$ become worse than before.
For the Wikipedia network, when $k \le 200$, the accuracy is above $90\%$ and we can get a $(1 \pm 0.1)$-approximation to $N_{uv}$, and when $k \ge 500$, the accuracy is above $80\%$ and we can get a $(1 \pm 0.2)$-approximation. For the Twitch network, the accuracy is about $70\%$-$80\%$ when $k \le 200$ and about $60\%$-$70\%$ when $k \ge 500$. Here $\rho_k$ is about $0.3$-$0.6$ when $k \le 200$ and is larger than $1$ when $k \ge 500$, 
%For the arbitrary order model, both the accuracy and $\rho_k$ are very close to $1$ for the Wikipedia network. For the Twitch network, the accuracy is about $70\%$-$80\%$, and $\rho_k$ is about $1.15$-$1.25$ when $k \le 200$.

%$\sum_{uv \in S_k} \hat{N}_{uv}$ / $\sum_{uv \in S_k} N_{uv}$ 
% \newpage



\begin{table*}[htbp]
	\centering  
	\caption{The accuracy of the oracle. The one above is for the Twitch network and the one below is for the Wikipedia network.}  
	\label{table:1}  
	
	\begin{tabular}{|c|c|c|c|c|c|}  
		\hline  
		& & & & &\\[-6pt]  
		& $k = 50$ & $k = 100$ & $k = 200$ & $k = 500$ & $k = 1000$\\  
		\hline
		& & & & &\\[-6pt]  
		Acc(adjacency) & 0.82 & 0.84& 0.86& 0.86& 0.838\\
		\hline
		& & & & &\\[-6pt]  
% 		$\sum_{uv \in S_k} \hat{R}_{uv}$ / $\sum_{uv \in S_k} R_{uv}$ 
		$\rho_k$(adjacency) & 0.121 & 0.146 & 0.198 & 0.245& 0.399 \\
		\hline
		& & & & &\\[-6pt]  
		Acc(arbitrary) & 0.84 & 0.74& 0.725& 0.69&0.629\\
		\hline
		& & & & &\\[-6pt]  
		$\rho_k$(arbitrary) & 0.334 & 0.461 & 0.658 & 1.22& 1.82 \\
		\hline
	\end{tabular}
	
	\begin{tabular}{|c|c|c|c|c|c|}  
		\hline  
		& & & & &\\[-6pt]  
		& $k = 50$ & $k = 100$ & $k = 200$& $k = 500$ & $k = 1000$\\  
		\hline
		& & & & &\\[-6pt]  
		Acc(adjacency) &0.98 &0.85 &0.78 &0.832& 0.88\\
		\hline
		& & & & &\\[-6pt]  
		%$\sum_{uv \in S_k} \hat{R}_{uv}$ / $\sum_{uv \in S_k} R_{uv}$ 
		$\rho_k$(adjacency) & 0.111 & 0.196& 0.365 &0.378 & 0.273\\
		\hline
		& & & & &\\[-6pt]  
		Acc(arbitrary) &0.94 & 0.93 & 0.925 & 0.854 & 0.806\\
		\hline
		& & & & &\\[-6pt]  
		$\rho_k$(arbitrary) & 0.060 & 0.074 & 0.114& 0.154 & 0.201\\
		\hline
	\end{tabular}
	
\end{table*}
